# Supplementary material for: Large Language Model-Guided Prediction Toward Quantum Materials Synthesis
Source: arXiv:2410.20976 source file (2024-10-28)
Supplement: Supplementary file 3 [file si_tab_lhs2rh_241004_01.tex]

\begin{longtable}{c|c|p{10cm}|c|c}
\caption{Selected examples of LHS2RHS}\label{tab_s_lhs2rhs}\\
No. &  Model & Text & GTS & JS \\
\Xhline{5\arrayrulewidth}
\endfirsthead
\multicolumn{4}{c}%
{{\tablename\ \thetable{} -- continued from previous page}} \\
No. &  Model & Text & GTS & JS \\
\hline
\endhead
\hline
\multicolumn{4}{r}{{Continued on next page}} \\
\endfoot
\hline
\endlastfoot
1 & True & 0.5 TiO2 + 0.66 SrCO3 + 0.25 Nb2O5 + 0.09 Li2CO3 $\rightarrow$ 1 Li0.18Sr0.66Ti0.5Nb0.5O3 + 0.75 CO2 & 1.0 & 1.0 \\
\hline
1 & LHS2RHS & 0.5 TiO2 + 0.66 SrCO3 + 0.25 Nb2O5 + 0.09 Li2CO3 $\rightarrow$  \textcolor{blue}{1 Li0.18Sr0.66Ti0.5Nb0.5O3 + 0.75 CO2} & 1.0 & 1.0 \\
\hline
1 & distilGPT2 & 0.5 TiO2 + 0.66 SrCO3 + 0.25 Nb2O5 + 0.09 Li2CO3 $\rightarrow$ \textcolor{blue}{0.09 Li2CO3 $\rightarrow$ 0.09 Li2CO3 $\rightarrow$ 0.09 Li} & 0.389 & 0.0 \\
\Xhline{5\arrayrulewidth}
2 & True & 0.204 CuO + 0.98 Fe2O3 + 0.153 NiO + 0.663 ZnO $\rightarrow$ 1 (Ni0.15Cu0.2Zn0.65O)1.02(Fe2O3)0.98 & 1.0 & 1.0 \\
\hline
2 & LHS2RHS & 0.204 CuO + 0.98 Fe2O3 + 0.153 NiO + 0.663 ZnO $\rightarrow$  \textcolor{blue}{1 (Ni0.15Cu0.2Zn0.65O)1.02(Fe2O3)0.98} & 1.0 & 1.0 \\
\hline
2 & distilGPT2 & 0.204 CuO + 0.98 Fe2O3 + 0.153 NiO + 0.663 ZnO $\rightarrow$ \textcolor{blue}{0.99 Fe2O3 + 0.09 Fe2O4 + 0.09 Fe2O5 } & 0.321 & 0.0 \\
\Xhline{5\arrayrulewidth}
3 & True & 3 CuO + 4 TiO2 + 1 CaCO3 $\rightarrow$ 1 CaCu3Ti4O12 + 1 CO2 & 1.0 & 1.0 \\
\hline
3 & LHS2RHS & 3 CuO + 4 TiO2 + 1 CaCO3 $\rightarrow$  \textcolor{blue}{1 CaCu3Ti4O12 + 1 CO2} & 1.0 & 1.0 \\
\hline
3 & distilGPT2 & 3 CuO + 4 TiO2 + 1 CaCO3 $\rightarrow$ \textcolor{blue}{1 CaCO3 $\rightarrow$ 1 CaCO3 $\rightarrow$} & 0.389 & 0.167 \\
\Xhline{5\arrayrulewidth}
4 & True & 2 MnO2 + 0.5 Li2CO3 $\rightarrow$ 1 LiMn2O4 + 0.5 CO2 + 0.25 O2 & 1.0 & 1.0 \\
\hline
4 & LHS2RHS & 2 MnO2 + 0.5 Li2CO3 $\rightarrow$  \textcolor{blue}{1 LiMn2O4 + 0.5 CO2 + 0.25 O2} & 1.0 & 1.0 \\
\hline
4 & distilGPT2 & 2 MnO2 + 0.5 Li2CO3 $\rightarrow$ \textcolor{blue}{MnO2 + 0.5 Li2CO3 $\rightarrow$ MnO2 + 0} & 0.477 & 0.182 \\
\Xhline{5\arrayrulewidth}
5 & True & 1 TiO2 + 1 BaCO3 $\rightarrow$ 1 BaTiO3 + 1 CO2 & 1.0 & 1.0 \\
\hline
5 & LHS2RHS & 1 TiO2 + 1 BaCO3 $\rightarrow$  \textcolor{blue}{1 BaTiO3 + 1 CO2} & 1.0 & 1.0 \\
\hline
5 & distilGPT2 & 1 TiO2 + 1 BaCO3 $\rightarrow$ \textcolor{blue}{TiO2 + 1 BaCO3 -} & 0.778 & 0.286 \\
\Xhline{5\arrayrulewidth}
6 & True & 0.5$*$x Gd2O3 + 0.5 Nb2O5 + 0.5-0.5$*$x Bi2O3 $\rightarrow$ 1 Bi1-xGdxNbO4 & 1.0 & 1.0 \\
\hline
6 & LHS2RHS & 0.5$*$x Gd2O3 + 0.5 Nb2O5 + 0.5-0.5$*$x Bi2O3 $\rightarrow$  \textcolor{blue}{1 Bi1-xGdxNbO4} & 1.0 & 1.0 \\
\hline
6 & distilGPT2 & 0.5$*$x Gd2O3 + 0.5 Nb2O5 + 0.5-0.5$*$x Bi2O3 $\rightarrow$ \textcolor{blue}{Gd2O3 $\rightarrow$ Gd2O3} & 0.6 & 0.0 \\
\Xhline{5\arrayrulewidth}
7 & True & 1 SiO2 + 3 SrCO3 $\rightarrow$ 1 Sr3SiO5 + 3 CO2 & 1.0 & 1.0 \\
\hline
7 & LHS2RHS & 1 SiO2 + 3 SrCO3 $\rightarrow$  \textcolor{blue}{1 Sr3SiO5 + 3 CO2} & 1.0 & 1.0 \\
\hline
7 & distilGPT2 & 1 SiO2 + 3 SrCO3 $\rightarrow$ \textcolor{blue}{SiO2 + 3 SrCO3 $\rightarrow$} & 0.655 & 0.25 \\
\Xhline{5\arrayrulewidth}
8 & True & 1 Al2O3 + 1 Ba(NO3)2 $\rightarrow$ 1 BaAl2O4 + 2 NO2 + 0.5 O2  & 1.0 & 1.0 \\
\hline
8 & LHS2RHS & 1 Al2O3 + 1 Ba(NO3)2 $\rightarrow$  \textcolor{blue}{1 BaAl2O4 + 2 NO2 + 0.5 O2 } & 1.0 & 1.0 \\
\hline
8 & distilGPT2 & 1 Al2O3 + 1 Ba(NO3)2 $\rightarrow$ \textcolor{blue}{1 Ba(NO4)2 $\rightarrow$ 1 Ba(NO5)2 $\rightarrow$} & 0.259 & 0.1 \\
\Xhline{5\arrayrulewidth}
9 & True & 1 SiO2 + 2 CaCO3 $\rightarrow$ 1 Ca2SiO4 + 2 CO2  & 1.0 & 1.0 \\
\hline
9 & LHS2RHS & 1 SiO2 + 2 CaCO3 $\rightarrow$  \textcolor{blue}{1 Ca2SiO4 + 2 CO2 } & 1.0 & 1.0 \\
\hline
9 & distilGPT2 & 1 SiO2 + 2 CaCO3 $\rightarrow$ \textcolor{blue}{SiO2 + 2 CaCO3 $\rightarrow$ } & 0.722 & 0.25 \\
\Xhline{5\arrayrulewidth}
10 & True & 1 FeC2O4·2H2O + 1 LiH2PO4 + 0.5 O2 $\rightarrow$ 1 LiFePO4 + 2 CO2 + 3 H2O & 1.0 & 1.0 \\
\hline
10 & LHS2RHS & 1 FeC2O4·2H2O + 1 LiH2PO4 + 0.5 O2 $\rightarrow$  \textcolor{blue}{1 LiFePO4 + 2 CO2 + 3 H2O} & 1.0 & 1.0 \\
\hline
10 & distilGPT2 & 1 FeC2O4·2H2O + 1 LiH2PO4 + 0.5 O2 $\rightarrow$ \textcolor{blue}{1 LiH2PO4 + 0.5 O2 $\rightarrow$ 1 L} & 0.483 & 0.167 \\
\Xhline{5\arrayrulewidth}
11 & True & 40 SiO2 + 20 TiO2 + 40 BaCO3 $\rightarrow$ 1 40BaO-20TiO2-40SiO2 + 40 CO2 & 1.0 & 1.0 \\
\hline
11 & LHS2RHS & 40 SiO2 + 20 TiO2 + 40 BaCO3 $\rightarrow$  \textcolor{blue}{1 40BaO-20TiO2-40SiO2 + 40 CO2} & 1.0 & 1.0 \\
\hline
11 & distilGPT2 & 40 SiO2 + 20 TiO2 + 40 BaCO3 $\rightarrow$ \textcolor{blue}{20 TiO2 + 40 BaCO3 $\rightarrow$ 20 TiO2 } & 0.714 & 0.222 \\
\Xhline{5\arrayrulewidth}
12 & True & 4 MgCO3 + 1 Nb2O5 $\rightarrow$ 1 Mg4Nb2O9 + 4 CO2 & 1.0 & 1.0 \\
\hline
12 & LHS2RHS & 4 MgCO3 + 1 Nb2O5 $\rightarrow$  \textcolor{blue}{1 Mg4Nb2O9 + 4 CO2} & 1.0 & 1.0 \\
\hline
12 & distilGPT2 & 4 MgCO3 + 1 Nb2O5 $\rightarrow$ \textcolor{blue}{MgCO3 + 1 Nb2O5 $\rightarrow$} & 0.691 & 0.25 \\
\Xhline{5\arrayrulewidth}
13 & True & 0.8+0.2$*$x TiO2 + 0.3$*$x CaCO3 + 1-0.3$*$x BaCO3 + 0.2-0.2$*$x ZrO2 $\rightarrow$ 1 (1-x)Ba(Zr0.2Ti0.8)O3-x(Ba0.7Ca0.3)TiO3 + 1 CO2 & 1.0 & 1.0 \\
\hline
13 & LHS2RHS & 0.8+0.2$*$x TiO2 + 0.3$*$x CaCO3 + 1-0.3$*$x BaCO3 + 0.2-0.2$*$x ZrO2 $\rightarrow$  \textcolor{blue}{1 (1-x)Ba(Zr0.2Ti0.8)O3-x(Ba0.7Ca0.3)TiO3 + 1 CO2} & 1.0 & 1.0 \\
\hline
13 & distilGPT2 & 0.8+0.2$*$x TiO2 + 0.3$*$x CaCO3 + 1-0.3$*$x BaCO3 + 0.2-0.2$*$x ZrO2 $\rightarrow$ \textcolor{blue}{0.3$*$x CaCO3 + 1-0.3$*$x CaCO3 + 1-0.3$*$x CaCO3 + 1-0} & 0.383 & 0.125 \\
\Xhline{5\arrayrulewidth}
14 & True & 1 ZnO + 0.2 Mg(OH)2·4MgCO3·6H2O $\rightarrow$ 1 ZnO-MgO + 0.8 CO2 + 1.4 H2O & 1.0 & 1.0 \\
\hline
14 & LHS2RHS & 1 ZnO + 0.2 Mg(OH)2·4MgCO3·6H2O $\rightarrow$  \textcolor{blue}{1 ZnO-MgO + 0.8 CO2 + 1.4 H2O} & 1.0 & 1.0 \\
\hline
14 & distilGPT2 & 1 ZnO + 0.2 Mg(OH)2·4MgCO3·6H2O $\rightarrow$ \textcolor{blue}{0.2 Mg(OH)2·4MgCO3·6H2O $\rightarrow$ 0.} & 0.238 & 0.0 \\
\Xhline{5\arrayrulewidth}
15 & True & 1 NiO + 0.5 V2O5 + 0.5 Li2CO3 $\rightarrow$ 1 LiNiVO4 + 0.5 CO2 & 1.0 & 1.0 \\
\hline
15 & LHS2RHS & 1 NiO + 0.5 V2O5 + 0.5 Li2CO3 $\rightarrow$  \textcolor{blue}{1 LiNiVO4 + 0.5 CO2} & 1.0 & 1.0 \\
\hline
15 & distilGPT2 & 1 NiO + 0.5 V2O5 + 0.5 Li2CO3 $\rightarrow$ \textcolor{blue}{0.5 Li2CO3 $\rightarrow$ 0.5 L} & 0.35 & 0.125 \\
\Xhline{5\arrayrulewidth}
16 & True & 2 NH4H2PO4 + 1 CaCO3 + 0.5 Y2O3 + 0.5 K2CO3 $\rightarrow$ 1 KCaY(PO4)2 + 1.5 CO2 + 3 H2O + 2 NH3  & 1.0 & 1.0 \\
\hline
16 & LHS2RHS & 2 NH4H2PO4 + 1 CaCO3 + 0.5 Y2O3 + 0.5 K2CO3 $\rightarrow$  \textcolor{blue}{1 KCaY(PO4)2 + 1.5 CO2 + 3 H2O + 2 NH3 } & 1.0 & 1.0 \\
\hline
16 & distilGPT2 & 2 NH4H2PO4 + 1 CaCO3 + 0.5 Y2O3 + 0.5 K2CO3 $\rightarrow$ \textcolor{blue}{0.5 K2CO3 $\rightarrow$ 0.5 K2CO3 $\rightarrow$ 0.5 K2CO3 $\rightarrow$ } & 0.175 & 0.0 \\
\Xhline{5\arrayrulewidth}
17 & True & 1 CaSO4 + 1 KCl $\rightarrow$ 1 KCaSO4Cl & 1.0 & 1.0 \\
\hline
17 & LHS2RHS & 1 CaSO4 + 1 KCl $\rightarrow$  \textcolor{blue}{1 KCaSO4Cl} & 1.0 & 1.0 \\
\hline
17 & distilGPT2 & 1 CaSO4 + 1 KCl $\rightarrow$ \textcolor{blue}{CaSO4 + 1 } & 0.45 & 0.25 \\
\Xhline{5\arrayrulewidth}
18 & True & 1 LiOH·H2O + 2 $\gamma$-MnOOH + 0.25 O2 $\rightarrow$ 1 LiMn2O4 + 2.5 H2O & 1.0 & 1.0 \\
\hline
18 & LHS2RHS & 1 LiOH·H2O + 2 $\gamma$-MnOOH + 0.25 O2 $\rightarrow$  \textcolor{blue}{1 LiMn2O4 + 2.5 H2O} & 1.0 & 1.0 \\
\hline
18 & distilGPT2 & 1 LiOH·H2O + 2 $\gamma$-MnOOH + 0.25 O2 $\rightarrow$ \textcolor{blue}{0.25} & 0.0 & 0.0 \\
\Xhline{5\arrayrulewidth}
19 & True & 1 FeC2O4·2H2O + 1 NH4H2PO4 + 0.5 Li2CO3 + 0.5 O2 $\rightarrow$ 1 LiFePO4 + 2.5 CO2 + 3.5 H2O + 1 NH3 & 1.0 & 1.0 \\
\hline
19 & LHS2RHS & 1 FeC2O4·2H2O + 1 NH4H2PO4 + 0.5 Li2CO3 + 0.5 O2 $\rightarrow$  \textcolor{blue}{1 LiFePO4 + 2.5 CO2 + 3.5 H2O + 1 NH3} & 1.0 & 1.0 \\
\hline
19 & distilGPT2 & 1 FeC2O4·2H2O + 1 NH4H2PO4 + 0.5 Li2CO3 + 0.5 O2 $\rightarrow$ \textcolor{blue}{1 NH4H2PO4 + 0.5 O2 $\rightarrow$ 1 NH4H2PO4 + 0} & 0.282 & 0.154 \\
\Xhline{5\arrayrulewidth}
20 & True & 1 SrCO3 + 1 RuO2 + 0.5 La2O3 + 1 MnO2 $\rightarrow$ 1 SrLaMnRuO6 + 1 CO2 + 0.25 O2 & 1.0 & 1.0 \\
\hline
20 & LHS2RHS & 1 SrCO3 + 1 RuO2 + 0.5 La2O3 + 1 MnO2 $\rightarrow$  \textcolor{blue}{1 SrLaMnRuO6 + 1 CO2 + 0.25 O2} & 1.0 & 1.0 \\
\hline
20 & distilGPT2 & 1 SrCO3 + 1 RuO2 + 0.5 La2O3 + 1 MnO2 $\rightarrow$ \textcolor{blue}{1} & 0.0 & 0.167 \\
\Xhline{5\arrayrulewidth}
21 & True & 1 Li2CuO2 + -1 Li $\rightarrow$ 1 LiCuO2 & 1.0 & 1.0 \\
\hline
21 & LHS2RHS & 1 Li2CuO2 + -1 Li $\rightarrow$  \textcolor{blue}{1 LiCuO2} & 1.0 & 1.0 \\
\hline
21 & distilGPT2 & 1 Li2CuO2 + -1 Li $\rightarrow$ \textcolor{blue}{Li $\rightarrow$ Li} & 0.167 & 0.0 \\
\Xhline{5\arrayrulewidth}
22 & True & 0.5 Fe2O3 + 0.5 La2O3 $\rightarrow$ 1 LaFeO3 & 1.0 & 1.0 \\
\hline
22 & LHS2RHS & 0.5 Fe2O3 + 0.5 La2O3 $\rightarrow$  \textcolor{blue}{1 LaFeO3} & 1.0 & 1.0 \\
\hline
22 & distilGPT2 & 0.5 Fe2O3 + 0.5 La2O3 $\rightarrow$ \textcolor{blue}{0.5 Fe2O} & 0.455 & 0.0 \\
\Xhline{5\arrayrulewidth}
23 & True & 0.4 PbO + 0.97 TiO2 + 0.006 (MgCO3)4·Mg(OH)2·5H2O + 0.6 SrCO3 $\rightarrow$ 1 Pb0.4Sr0.6(Ti0.97Mg0.03)O2.97 + 0.624 CO2 + 0.036 H2O & 1.0 & 1.0 \\
\hline
23 & LHS2RHS & 0.4 PbO + 0.97 TiO2 + 0.006 (MgCO3)4·Mg(OH)2·5H2O + 0.6 SrCO3 $\rightarrow$  \textcolor{blue}{1 Pb0.4Sr0.6(Ti0.97Mg0.03)O2.97 + 0.624 CO2 + 0.036 H2O} & 1.0 & 1.0 \\
\hline
23 & distilGPT2 & 0.4 PbO + 0.97 TiO2 + 0.006 (MgCO3)4·Mg(OH)2·5H2O + 0.6 SrCO3 $\rightarrow$ \textcolor{blue}{0.005 (MgCO3)4·Mg(OH)2·5H2O + 0.6 SrCO3 $\rightarrow$ 0.005 (MgCO3} & 0.488 & 0.077 \\
\Xhline{5\arrayrulewidth}
24 & True & 2 C + 1 Si + 3 Ti $\rightarrow$ 1 Ti3SiC2 & 1.0 & 1.0 \\
\hline
24 & LHS2RHS & 2 C + 1 Si + 3 Ti $\rightarrow$  \textcolor{blue}{1 Ti3SiC2} & 1.0 & 1.0 \\
\hline
24 & distilGPT2 & 2 C + 1 Si + 3 Ti $\rightarrow$ \textcolor{blue}{1 Si + 3 } & 0.036 & 0.2 \\
\Xhline{5\arrayrulewidth}
25 & True & 6 Na2CO3 + 6 TiO2 $\rightarrow$ 1 Na12(TiO3)6 + 6 CO2 & 1.0 & 1.0 \\
\hline
25 & LHS2RHS & 6 Na2CO3 + 6 TiO2 $\rightarrow$  \textcolor{blue}{1 Na12(TiO3)6 + 6 CO2} & 1.0 & 1.0 \\
\hline
25 & distilGPT2 & 6 Na2CO3 + 6 TiO2 $\rightarrow$ \textcolor{blue}{Na2CO3 + 6 TiO2 $\rightarrow$ Na} & 0.408 & 0.222 \\
\Xhline{5\arrayrulewidth}
26 & True & 0.5 La2O3 + 1 Mg(OH)2 + 11 Al(OH)3 $\rightarrow$ 1 LaMgAl11O19 + 17.5 H2O  & 1.0 & 1.0 \\
\hline
26 & LHS2RHS & 0.5 La2O3 + 1 Mg(OH)2 + 11 Al(OH)3 $\rightarrow$  \textcolor{blue}{1 LaMgAl11O19 + 17.5 H2O } & 1.0 & 1.0 \\
\hline
26 & distilGPT2 & 0.5 La2O3 + 1 Mg(OH)2 + 11 Al(OH)3 $\rightarrow$ \textcolor{blue}{1 Mg(OH)3 $\rightarrow$ 1 Mg(OH)3 $\rightarrow$} & 0.3 & 0.143 \\
\Xhline{5\arrayrulewidth}
27 & True & 5 TiO2 + 1 Nb2O5 + 5 Li2CO3 $\rightarrow$ 1 5Li2O-1Nb2O5-5TiO2 + 5 CO2 & 1.0 & 1.0 \\
\hline
27 & LHS2RHS & 5 TiO2 + 1 Nb2O5 + 5 Li2CO3 $\rightarrow$  \textcolor{blue}{1 5Li2O-1Nb2O5-5TiO2 + 5 CO2} & 1.0 & 1.0 \\
\hline
27 & distilGPT2 & 5 TiO2 + 1 Nb2O5 + 5 Li2CO3 $\rightarrow$ \textcolor{blue}{1 Nb2O5 + 5 Li2CO3 $\rightarrow$ 1 Nb2O} & 0.593 & 0.333 \\
\Xhline{5\arrayrulewidth}
28 & True & 1 SiO2 + 0.5 Fe2O3 + 1 Li2CO3 $\rightarrow$ 1 Li2FeSiO4 + 1 CO2 + 0.25 O2 & 1.0 & 1.0 \\
\hline
28 & LHS2RHS & 1 SiO2 + 0.5 Fe2O3 + 1 Li2CO3 $\rightarrow$  \textcolor{blue}{1 Li2FeSiO4 + 1 CO2 + 0.25 O2} & 1.0 & 1.0 \\
\hline
28 & distilGPT2 & 1 SiO2 + 0.5 Fe2O3 + 1 Li2CO3 $\rightarrow$ \textcolor{blue}{SiO3 $\rightarrow$ SiO3 $\rightarrow$ SiO3 $\rightarrow$ SiO3 } & 0.25 & 0.0 \\
\Xhline{5\arrayrulewidth}
29 & True & 1 MoO3 + 1 Cs2CO3 $\rightarrow$ 1 Cs2MoO4 + 1 CO2 & 1.0 & 1.0 \\
\hline
29 & LHS2RHS & 1 MoO3 + 1 Cs2CO3 $\rightarrow$  \textcolor{blue}{1 Cs2MoO4 + 1 CO2} & 1.0 & 1.0 \\
\hline
29 & distilGPT2 & 1 MoO3 + 1 Cs2CO3 $\rightarrow$ \textcolor{blue}{Cs2CO3 $\rightarrow$ Cs2CO3 } & 0.421 & 0.0 \\
\Xhline{5\arrayrulewidth}
30 & True & 7 NH4H2PO4 + 10 CaCO3 + 0.5 K2CO3 $\rightarrow$ 1 Ca10K(PO4)7 + 10.5 CO2 + 10.5 H2O + 7 NH3 & 1.0 & 1.0 \\
\hline
30 & LHS2RHS & 7 NH4H2PO4 + 10 CaCO3 + 0.5 K2CO3 $\rightarrow$  \textcolor{blue}{1 Ca10K(PO4)7 + 10.5 CO2 + 10.5 H2O + 7 NH3} & 1.0 & 1.0 \\
\hline
30 & distilGPT2 & 7 NH4H2PO4 + 10 CaCO3 + 0.5 K2CO3 $\rightarrow$ \textcolor{blue}{0.5 K2CO3 $\rightarrow$ 0.5 K2CO3 $\rightarrow$ 0.5 K2CO3 $\rightarrow$ 0.5 } & 0.146 & 0.0 \\
\Xhline{5\arrayrulewidth}
\end{longtable}
